# Supplementary material for: Polarimetric BSSRDF Acquisition of Dynamic Faces
Source: arXiv:2501.01980 source file (2024-12-29)
Supplement: Supplementary file 1 [file appendix.tex]

\appendix
\section{Appendix}
